# Supplementary material for: Screw dislocation that converts p-type GaN to n-type: Microscopic study on the Mg condensation and the leakage current in p-n diodes
Source: arXiv:2004.06876 ancillary file (2020-04-15)
Supplement: Supplementary file 1 [file supplement.pdf]

# Supplementary Information

# Screw dislocation that converts p-type GaN to n-type: Microscopic study on the Mg condensation and the leakage current in p-n diodes

T. Nakano,[1, a)] Y. Harashima,[2, b)] K. Chokawa,[2] K. Shiraishi,[1, 2] A. Oshiyama,[2] Y. Kangawa,[3] S. Usami,[1] N. Mayama,[4] K. Toda,[4] A. Tanaka,[2] Y. Honda,[1, 2] and H. Amano[1, 2]

[1)] *Graduate School of Engineering, Nagoya University, Nagoya 464-8601, Japan*
[2)] *Institute of Materials and Systems for Sustainability, Nagoya University, Nagoya 464-8601, Japan*
[3)] *Research Institute for Applied Mechanics, Kyushu University, Fukuoka 816-8580, Japan*
[4)] *Toshiba Nanoanalysis Corporation, Yokohama 235-8522, Japan*

(Dated: 13 April 2020)

### SA. Core structures of [0001] screw dislocations in GaN

In previous first-principles calculations[1], the electronic structures of 1/3[11-20] edge dislocations in GaN has been examined and the obtained density of states near the energy gap suggests that edge dislocations do not cause the leakage current. The electronic properties and stabilities of the core structures of the [0001] screw dislocation have been also reported in literature.[2–8] Belabbas *et al.*[2,8,9], Northrup[3,5] and Pizzagalli *et al.*[10] have examined the stabilities of four distinct types of the core configurations using first-principles calculations: a filled core[8,9] in which all Ga and N atoms remain in the core region, an open core[3] in which those Ga and N atoms are removed from the core region, a Ga-filled core[3] in which N atoms are partially removed from the core region, and a N-filled core[10] in which Ga atoms are partially removed from the core region. Those calculations suggest that the dislocations with the open core, the Ga-filled core, and the half Ga-filled core where three N atoms are removed are likely to appear during the epitaxial growth under certain conditions.[3–7] Belabbas *et al.*[2,8,11], Northrup[3], Matsubara *et al*[6,7]. and Blumenau *et al.*[12] have examined the electronic structure of such dislocation cores and argue that the possible core structures may result in some energy levels in the band gap. These results suggest that the performance and the reliability of GaN power devices depends on the growth conditions.

In this work, we have performed systematic search for the most stable dislocation cores with possible 16 stoichiometric ratios of Ga and N in the core region based on the density-functional theory. In the previous calculations, the systems examined contain at most 200 atoms. This system size should be larger to relax the artificial strain caused by the boundary conditions. In our supercell model, each cell contains about 900 atoms in total and is separated from its adjacent cells by the vacuum region on the lateral surface: i.e., the rod-shape cell.

We consider 16 distinct core configurations as follows. We first prepare filled cores. Depending on the position of the screw dislocation line along [0001], there are two types of the dislocation cores: In one type which we call single core[8], the dislocation line is at the center of the single hexagon, whereas in the other type which we call double core[9], the dislocation line is at the middle of the central bond of double hexagons (see Fig. 2(a) in the main text). We next prepare partially filled and also open cores by removing several atoms from those filled cores. It is expected that removing some atoms relaxes the strongly distorted covalent bonds.[5–7] We use the notation $\mathrm{S}(n|m)$ or $\mathrm{D}(n|m)$ which denote the core prepared by removing $n$ Ga atoms and $m$ N atoms from the single or double filled core (Fig. 2(a)) (The notation follows the notation in Fig. 1 of Pizzagalli *et al.*[10], but the sign is opposite). We have performed the full structural optimization for 16 possible distinct dislocation cores, D(0|0), D(0|1), D(0|2), D(0|4), D(0|6), D(1|0), D(2|0), D(2|2), S(0|0), S(0|3), S(0|6), S(0|12), S(3|0), S(6|0), S(6|3), and S(6|6).

The stability of the dislocation cores is evaluated by the formation energy $E_\mathrm{f}$ defined as,

$$E_\mathrm{f} = E - E^\mathrm{ref} - \mu_\mathrm{N}\Delta n_\mathrm{N} - \mu_\mathrm{Ga}\Delta n_\mathrm{Ga}. \quad \text{(S1)}$$

Here, $E$ and $E^\mathrm{ref}$ are the total energies of the supercell with the dislocation core and of the reference model, respectively. In this paper, we choose the D(0|0) core as a reference. $\Delta n_\mathrm{N} = n_\mathrm{N} - n_\mathrm{N}^\mathrm{ref}$ $(\Delta n_\mathrm{Ga} = n_\mathrm{Ga} - n_\mathrm{Ga}^\mathrm{ref})$ where $n_\mathrm{N}$ $(n_\mathrm{Ga})$ and $n_\mathrm{N}^\mathrm{ref}$ $(n_\mathrm{Ga}^\mathrm{ref})$ are the numbers of N (Ga) atoms in the supercells corresponding to $E$ and $E^\mathrm{ref}$, respectively. The chemical potentials satisfy the equilibrium condition, $\mu_\mathrm{GaN} = \mu_\mathrm{Ga} + \mu_\mathrm{N} = \mu_\mathrm{Ga}^0 + \mu_\mathrm{N}^0 + \Delta H_\mathrm{f}^0$. Here, $\Delta H_\mathrm{f}^0$ is the formation enthalpy of GaN, $\mu_\mathrm{Ga}^0$ is the chemical potential of $\alpha$-Ga metal, and $\mu_\mathrm{N}^0$ is the chemical potential of N in the $N_2$ molecule. Thus, $\mu_\mathrm{Ga} - \mu_\mathrm{Ga}^0$ ranges from $\Delta H_\mathrm{f}^0 = -0.92$ eV (Ga-poor condition) to 0.0 eV (Ga-rich condition).

---

[a)] Electronic mail: nakano.takashi@h.nagoya-u.jp
[b)] Corresponding author: yosuke.harashima@imass.nagoya-u.ac.jp

Figure 2(b) shows the calculated formation energy of each core structure of the [0001] screw dislocation as a function of $\mu_{Ga}$. For the filled core structures, the D(0|0) core is more stable than the S(0|0) core. For structures in which several Ga atoms and N atoms are removed, the N removed structures tend to be more stable than filled core models. In such cases, the strain is partially relaxed. In gallium-rich conditions, the S(0|6) core is the most stable, which is consistent with other reports.[3,6,7] In N-rich conditions, the D(0|2) core is the most stable. In the intermediate region of $\mu_{Ga}$, the S(0|3) core is also stable. It is noteworthy that even in the N-rich (Ga-poor) condition, the Ga-filled cores are energetically favorable. In contrast to present results, some previous calculations[3,6,7] show that the open core is stable. This discrepancy is considered to be due to the difference in the cell size and the existence of the vacuum region in the calculation.

We have examined the electronic structures of the S(0|6), the S(0|3), and the D(0|2) cores and found that these core structures induces energy levels in the band gap. These levels have been also obtained in the previous calculations.[3,6,7] In experiments, GaN samples grown in both Ga-rich and N-rich conditions have shown reverse leakage.[13–15] In our main text, we focus on the stable cores, the D(0|2), the S(0|6) and the S(0|3) (Fig. 4), and we clarify the interaction between each screw dislocation and Mg impurity states.

## SB. Procedure of atom probe tomography (APT) and setting up samples

The APT analysis enables us to understand the three-dimensional condensations of constituent atomic species and their amount by combing field-ion microscopy and time-of-flight mass spectrometry. The sample containing screw dislocations under an etch-pit is formed into a needle shape, and a pulsed laser is applied to evaporate one atomic layer at a time from the apex of tip. The flight position and time-of-flight of atoms that have been evaporated in the high electric field are detected by the 2D detector. A three-dimensional atomic map of the probe is constructed by the stacking this information.

Here, we simply describe the procedure of fabrication and evaluation of the sample: a more detailed explanation of the procedures is described in the previous work.[16] First, we have fabricated a vertical p-n diode having an n-type drift layer and p-type layer ([Mg]>$10^{19}$ $cm^{-3}$) grown by metal-organic vapor phase epitaxy (MOVPE) on a free-standing GaN substrate. The reverse I-V characteristics of this p-n diode is measured by using a semiconductor parameter analyzer and we have observed that a breakdown occurs at $-650$ V with a relatively high reverse leakage current. Then, the leakage position was observed by emission microscopy. The density of the observed leakage spots was $5 \times 10^5$ $cm^{-2}$ and this was about 1/20 of the total threading dislocation density. Next, the p-type layer was etched to expose the drift layer near the p-n junction and three types of etch pits (large, medium, and small) are then formed at the dislocation spots by dipping the exposed drift layer in molten KOH. The etch pit size and shape reflect the dislocation type[17–24] and the dislocation types are then identified on the basis of the large-angle convergent-beam electron diffraction (LACBED) method.[25,26] We have performed APT analysis for the medium pits, which are determined as TSD by LACBED method, having an observable leakage current.[27]


[1] T. Nakano, M. Araidai, K. Shiraishi, A. Tanaka, Y. Honda, and H. Amano, ECS Transactions **86**, 41–49 (2018).
[2] I. Belabbas, J. Chen, and G. Nouet, Comput. Mater. Sci. **90**, 71–81 (2014).
[3] J. E. Northrup, Appl. Phys. Lett. **78**, 2288 (2001).
[4] R. Gröger, L. Leconte, and A. Ostapovets, Comp. Mater. Sci. **99**, 195–202 (2015).
[5] J. E. Northrup, Phys. Rev. B **66**, 045204 (2002).
[6] M. Matsubara, J. Godet, L. Pizzagalli, and E. Bellotti, Appl. Phys. Lett. **103**, 262107 (2013).
[7] M. Matsubara, L. Pizzagalli, and E. Bellotti, Phys. Status Solidi C **11**, 521–524 (2014).
[8] I. Belabbas, M. Belkhir, Y. Lee, A. Béré, P. Ruterana, J. Chen, and G. Nouet, Comput. Mater. Sci. **37**, 410 (2006).
[9] I. Belabbas, J. Chen, and G. Nouet, Comput. Mater. Sci. **51**, 206–216 (2011).
[10] L. Pizzagalli, I. Belabbas, J. Kioseoglou, and J. Chen, Phys. Rev. Materials **2**, 064607 (2018).
[11] I. Belabbas, P. Ruterana, J. Chen, and G. Nouet, Philos. Mag. **86**, 2241 (2006).
[12] A. T. Blumenau, C. J. Fall, J. Elsner, R. Jones, M. I. Heggie, and T. Frauenheim, Phys. Status Solidi (c) **0**, 1684 (2003).
[13] J. W. P. Hsu, M. J. Manfra, S. N. G. Chu, C. H. Chen, L. N. Pfeiffer, and R. J. Molnar, Appl. Phys. Lett. **78**, 3980–3982 (2001).
[14] J. W. P. Hsu, M. J. Manfra, R. J. Molnar, B. Heying, and J. S. Speck, Appl. Phys. Lett. **81**, 79 (2002).
[15] J. J. M. Law, E. T. Yu, G. Koblmüller, F. Wu, and J. S. Speck, Appl. Phys. Lett. **96**, 102111 (2010).
[16] S. Usami, N. Mayama, K. Toda, A. Tanaka, M. Deki, S. Nitta, Y. Honda, and H. Amano, Appl. Phys. Lett. **114**, 232105 (2019).
[17] S. K. Hong, B. J. Kim, H. S. Park, Y. Park, S. Y. Yoon, and T. I. Kim, J. Cryst. Growth **191**, 275 (1998).
[18] T. Hino, S. Tomiya, T. Miyajima, K. Yanashima, S. Hashimoto, and M. Ikeda, Appl. Phys. Lett. **76**, 3421 (2000).
[19] J. L. Weyher, Superlattices Microstruct. **40**, 279 (2006).
[20] J. Chen, J. F. Wang, H. Wang, J. J. Zhu, S. M. Zhang, D. G. Zhao, D. S. Jiang, H. Yang, U. Jahn, and K. H. Ploog, Semicond. Sci. Technol. **21**, 1229 (2006).
[21] J. L. Weyher, S. Lazar, L. Macht, Z. Liliental-Weber, R. J. Molnar, S. Müller, V. G. M. Sivel, G. Nowak, and I. Grzegory, J. Cryst. Growth **305**, 384 (2007).
[22] L. Lu, Z. Y. Gao, B. Shen, F. J. Xu, S. Huang, Z. L. Miao, Y. Hao, Z. J. Yang, G. Y. Zhang, X. P. Zhang, J. Zu, and D. P. Yu, J. Appl. Phys. **104**, 123525 (2008).
[23] L. Zhang, Y. Shao, W. X. Hao, X. Chen, S. Qu, and X. Xu, J. Alloys Compd. **504**, 186 (2010).
[24] Y. Yao, Y. Ishikawa, Y. Sugawara, D. Yokoe, M. Sudo, N. Okada, and K. Tadatomo, Superlattices Microstruct. **99**, 83 (2016).
[25] M. Tanaka, M. Terauchi, and T. Kaneyama, Microscopy **40**, 211–220 (1991).
[26] D. Cherns and J.-P. Morniroli, Ultramicroscopy **53**, 167–180 (1994).
[27] S. Usami, Y. Ando, A. Tanaka, K. Nagamatsu, M. Deki, M. Kushimoto, S. Nitta, Y. Honda, H. Amano, Y. Sugawara, Y. Z. Yao, and Y. Ishikawa, Appl. Phys. Lett. **112**, 182106 (2018).
